# Supplementary material for: ShapleyLaw: A Game-Theoretic Approach to Multilingual Scaling Laws
Source: arXiv:2603.17945 source file (2026-09-19)
Supplement: Supplementary file 1 [file MCSV.tex]

\subsection{Monte Carlo Approximation of Shapley Values}
\label{app:mcsv}

\paragraph{Why approximation is needed.}
For a MPG, the definition of SV of language $i$ on task $j$ is
\begin{align*}
\sv_{i,j}(\mpg) = \textstyle\sum_{S \subseteq \languageset \setminus{i}} W(S)\cdot \improvement(S)
\end{align*}
where $W(S)=\frac{|S|!(K-|S|-1)!}{K!}$ and $\improvement(S)=\payoff_{j}(S\cup{i})-\payoff_{j}(S)$.
Computing such a SV exactly requires utility evaluation on all non-empty coalitions, which entails pre-training $2^K-1$ models for $K$ language candidates.
This cost is already substantial for moderate $K$, and becomes prohibitive in multilingual pre-training where each utility evaluation itself requires training and validating a model.
Therefore, approximation is necessary for scalable SV estimation.

\paragraph{Monte Carlo (MC) Approximation.}
A standard approximation strategy is permutation-based MC sampling.
Instead of enumerating all subsets, we sample $m$ random permutations of the $K$ languages and estimate each language's SV by averaging its marginal contribution over the sampled permutations.

Formally, let $\pi$ be a uniformly random permutation of the language set $\languageset$, and let $P_i^\pi$ denote the set of languages appearing before language $i$ in $\pi$.
Then the SV of $i$ can be written as the expectation
\begin{equation}
\sv_{i, j}
=
\mathbb{E}_{\pi}
\left[
\payoff_j(P_i^\pi \cup \{i\}) - \payoff_j(P_i^\pi)
\right].
\label{eq:sv_perm}
\end{equation}
MC approximation replaces the expectation in Eq.~\ref{eq:sv_perm} with an empirical average over $T$ permutations:
\begin{equation*}
\hat{\phi}_{i, j}^{SV}
=
\frac{1}{T}
\sum_{t=1}^{T}
\left[
\payoff_j(P_i^{\pi_t} \cup \{i\}) - \payoff_j(P_i^{\pi_t})
\right].
\label{eq:sv_mc}
\end{equation*}
This estimator is unbiased and converges to the exact SV as $T$ increases.

\begin{algorithm}[t]
\small
\caption{Monte Carlo Approximation}
\label{alg:mcsv}
\begin{algorithmic}[1]
\Require Language set $\languageset$, payoff function $\payoff_j(\cdot)$, number of permutations $T$
\Ensure Approximate SVs $\hat{\phi}_{1,j},\dots,\hat{\phi}_{K,j}$
\For{$i=1$ to $K$}
    \State $\hat{\phi}_{i,j} \gets 0$
\EndFor
\For{$t=1$ to $T$}
    \State Sample a random permutation $\pi_t$ of $\languageset$
    \State $S \gets \emptyset$
    \For{$k=1$ to $K$}
        \State $i \gets \pi_t(k)$
        \State $\Delta \gets \payoff_j(S \cup \{i\}) - \payoff_j(S)$
        \State $\hat{\phi}_{i,j} \gets \hat{\phi}_{i,j} + \Delta$
        \State $S \gets S \cup \{i\}$
    \EndFor
\EndFor
\For{$i=1$ to $K$}
    \State $\hat{\phi}_{i,j} \gets \hat{\phi}_{i,j} / T$
\EndFor
\State \textbf{return} $\hat{\phi}_{1,j},\dots,\hat{\phi}_{K,j}$
\end{algorithmic}
\end{algorithm}

\paragraph{Choice of $T$.}
~\citet{jia2019towards} found that when the number of permutations is 
\begin{align}
\label{eq:permutation}
    T(\epsilon, \delta) = [2 (\maxpayoff_j)^2 K / \epsilon^2] / \log(2K / \delta)
\end{align}
where $\maxpayoff_j$ denotes the test loss on language $j$ when the model has not been pretrained (i.e., the maximum possible payoff for task $\task_j$), the MC approximation achieves an $(\epsilon, \delta)$-approximation, i.e.,
\begin{align}
    \Pr\!\left[\left|\hat{\phi}_{\cdot, j}^{SV} - \sv_{\cdot, j}\right|_2 \ge 1 - \delta
\right] \le \epsilon
\label{eq:hoeffding}
\end{align}
where $\sv_{\cdot, j} = [\sv_{1, j}, \dots, \sv_{K, j}]$.
Therefore, given an approximation configuration $(\epsilon, \delta)$, we can determine the number of permutations $T$ using Formula~\ref{eq:permutation}.

\paragraph{Computational Complexity.}
For each permutation, the MC approximation requires evaluating $K$ pretrained models. 
Therefore, when performing $T(\epsilon, \delta)$ permutations, the MC approximation requires evaluating a total of $K\cdot T(\epsilon, \delta) = O(K^2 \log(K))$ models.
Thus, for MC approximation, we need to pretrain $O(K^2 \log(K))$ models for evaluation, which is significantly less complex than the $O(2^K)$ models required for exact SV computation.
Note that there is repeated evaluation of the same pretrained models across different permutations. 
Therefore, the number of pretrained models required for MC approximation is usually significantly smaller than the number of model evaluations $K\cdot T(\epsilon, \delta)$.

\subsection{Additional Experiments on SV Approximation}
\begin{figure*}[t]
  \centering
  \includegraphics[width=0.48\linewidth]{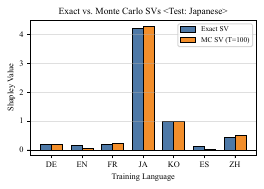}
  \hfill
  \includegraphics[width=0.48\linewidth]{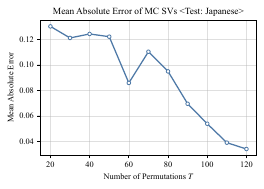}
  
  \caption{\textbf{Experimental Results of MC Approximation for SVs (Group: Japanese).} We use the SV group $\sv_{\texttt{ja}}$ as a representative case study. \textbf{Left}: We compare exact SVs $\sv_{\texttt{ja}}$ (blue bars) with MC approximations (orange bars) using $T=100$ samples. The approximated values closely match the exact SVs (e.g., $\sv_{\texttt{ja},\texttt{ja}}=4.199$ vs.\ $\hat{\phi}^{SV}_{\texttt{ja},\texttt{ja}}=4.272$) while preserving the same ranking. \textbf{Right}: We report the mean absolute error (MAE) as the sampling budget $m$ varies from 20 to 120. The approximation error decreases steadily as the number of samples increases.}
  \label{fig:MCSV}
\end{figure*}


We apply MC approximation to the multilingual pre-training game with
\[
\languageset=\{\texttt{en}, \texttt{de}, \texttt{fr}, \texttt{es}, \texttt{zh}, \texttt{ja}, \texttt{ko}\}
\]
where $K=7$.
In the exact setting, computing the full SV matrix requires evaluating all $2^7-1=127$ non-empty coalitions, i.e., pre-training 127 models.
Although this cost is still manageable for $K=7$, it already illustrates the exponential growth of exact SV estimation and serves as a controlled benchmark for approximation quality.

In our comparison experiments, we first use the SV group $\sv_{\texttt{ja}}$ as a representative case study and compare exact SVs against MC approximated SVs.
First, we fix the number of samples to $m=100$ and plot the approximated SVs against the exact SVs for $\sv_{\texttt{ja}}$.
Figure~\ref{fig:MCSV} directly shows that MC sampling can recover the overall SV pattern with substantially fewer utility evaluations than full coalition enumeration.
Second, we vary the sampling number from $m=20$ to $m=120$ and plot the mean absolute error (MAE)
\(
|\hat{\phi}_{i,\texttt{ja}}^{SV(m)}-\sv_{i,\texttt{ja}}|
\)
to examine convergence behavior.
The resulting trend shows that the approximation error decreases as the sampling budget increases, consistent with the concentration behavior in Eq.~\ref{eq:hoeffding}. 


\begin{figure}[t]
    \includegraphics[width=\linewidth]{Figure/NormalizedSV_heatmap_MC_50.pdf}
   \caption {\textbf{Monte Carlo Approximated Normalized SVs Matrix.} The results show that MC–approximated SVs still capture cross-lingual transfer effects, with only a slight reduction in accuracy.}
   \label{fig:MC_sv_matrix}
\end{figure}

These results suggest that MC approximation is an effective surrogate for exact SV computation in multilingual pre-training.
For small language sets such as $K=7$, it provides a useful accuracy--efficiency trade-off and can be directly validated against exact SVs.
For larger multilingual candidate pools, where exact enumeration becomes infeasible due to the $2^K-1$ training cost, the benefit of MC approximation becomes even more pronounced.
Overall, MC approximation offers a practical and scalable approach to SV estimation, especially when the total number of candidate languages is large.
